# Supplementary material for: A simple method to find temporal overlap between THz and X-ray pulses using X-ray-induced carrier dynamics in semiconductors
Source: arXiv:2410.03206 source file (2024-12-19)
Supplement: Supplementary file 1 [file XrayTHz_manuscript_SM_submit.pdf]

# Supplementary material

## A simple method to find temporal overlap between THz and x-ray pulses using x-ray-induced carrier dynamics in semiconductors

Yuya Kubota<sup>1</sup>, Takeshi Suzuki<sup>2</sup>, Shigeki Owada<sup>3,1</sup>, Kenji Tamasaku<sup>1</sup>,  
Hitoshi Osawa<sup>3</sup>, Tadashi Togashi<sup>3,1</sup>, Kozo Okazaki<sup>2</sup>, and Makina Yabashi<sup>1,3</sup>

<sup>1</sup>*RIKEN SPring-8 Center, 1-1-1 Kouto, Sayo, Hyogo 679-5148, Japan*

<sup>2</sup>*Institute for Solid State Physics, The University  
of Tokyo, Kashiwa, Chiba 277-8581, Japan*

<sup>3</sup>*Japan Synchrotron Radiation Research Institute (JASRI),  
1-1-1 Kouto, Sayo, Hyogo 679-5198, Japan*

(Dated: October 2, 2024)

## I. SIMULATION WITH A DIFFUSION EQUATION

We simulated carrier diffusion to investigate how relaxation time depends on sample thickness, as shown in Fig. 2 in the main text. The diffusion equation in the depth direction ( $z$ ) is described by

$$\frac{\partial N(z, t)}{\partial t} = D \frac{\partial^2}{\partial z^2} N(z, t) - \frac{N(z, t)}{\tau_0}, \quad (\text{S1})$$

where  $N(z, t)$  is carrier density at position  $z$  and time  $t$ ,  $D$  is diffusion coefficient, and  $\tau_0$  is the lifetime. The initial condition is determined by the excitation profile by x-ray pulses by

$$N(z, 0) = N_0 \exp\left(-\frac{z}{d}\right), \quad (\text{S2})$$

where  $N_0$  is the carrier density at the surface ( $z = 0$ ) and  $d$  is the penetration depth. The boundary conditions are determined by the surface recombinations as [1]

$$\frac{\partial N(0, t)}{\partial z} = \frac{S}{D} N(0, t), \text{ and } \frac{\partial N(L, t)}{\partial z} = -\frac{S}{D} N(L, t), \quad (\text{S3})$$

where  $S$  is the surface recombination velocity, and  $z = L$  is the boundary at the end of the sample. In the case of Si, we use the suitable values to the current experimental conditions as  $D = 18 \text{ cm}^2/\text{s}$  [2],  $\tau_0 = 30 \text{ } \mu\text{s}$  [3],  $d = 133 \text{ } \mu\text{m}$  [4], and  $S = 5 \times 10^3 \text{ cm/s}$  [5], respectively. Figures S1(a) and S1(b) show the calculated results of carrier density as a function of delay time and depth with the thickness  $L$  of 200 and 1000  $\mu\text{m}$ . We observed that carriers reach  $z = L$  before the carrier lifetime when  $L = 200 \text{ } \mu\text{m}$ . This accelerates the decay of carriers due to the surface recombination process. Conversely, when  $L = 1000 \text{ } \mu\text{m}$ , carriers recombine before reaching  $z = L$ . To simulate how the transmission of THz pulses changes due to such spatial and temporal distributions, we approximately model this inhomogeneously distributed situation. Figure S1(c) shows the schematic picture of the model. We discretized the depth profile as sample  $z = z_k$  ( $k = 1 - N$ ). Then, the transmittance of THz is described by

$$E_{\text{out}} = \left( \frac{2n(z_1)}{n(z_1) + 1} \sum_{k=1}^N \exp\left(i \frac{n(z_k) \omega \Delta z}{c}\right) \frac{2}{n(z_N) + 1} \right) E_{\text{in}}, \quad (\text{S4})$$

where  $n(z_k)$  is the refractive index at  $z = z_k$ ,  $\omega$  is the angular frequency,  $c$  is the speed of the light, and  $\Delta z = L/N$ . We use  $N = 500$ . We used the Drude model to calculate the dielectric function as

$$\epsilon(z_k) = \epsilon_b - i \frac{f_{pl}(z_k)^2}{f + i\gamma}, \quad (\text{S5})$$

where  $\epsilon_b = 11.7$  is the background dielectric constant for Si [6] and  $\gamma$  is the damping rate of the free carrier. We set  $f_{pl}(z = 0) = 4$  THz from the excitation density,  $f = 1$  THz as a dominant frequency component [Fig. 2(c)], and  $\gamma = 1$  THz for the typical value of the free carrier in such an excitation density [7]. The refractive index  $n$  is related to the dielectric function as  $n = \sqrt{\epsilon}$ . Figure S1(d) displays simulated results of the transmission of THz pulses,  $T = |E_{\text{out}}/E_{\text{in}}|^2$ , for the sample thickness  $L = 200, 500$ , and  $1000 \mu\text{m}$ . It is evident that the relaxation time of transmission increases as the thickness becomes larger, consistent with the experimental results shown in Fig. 2 in the main text.

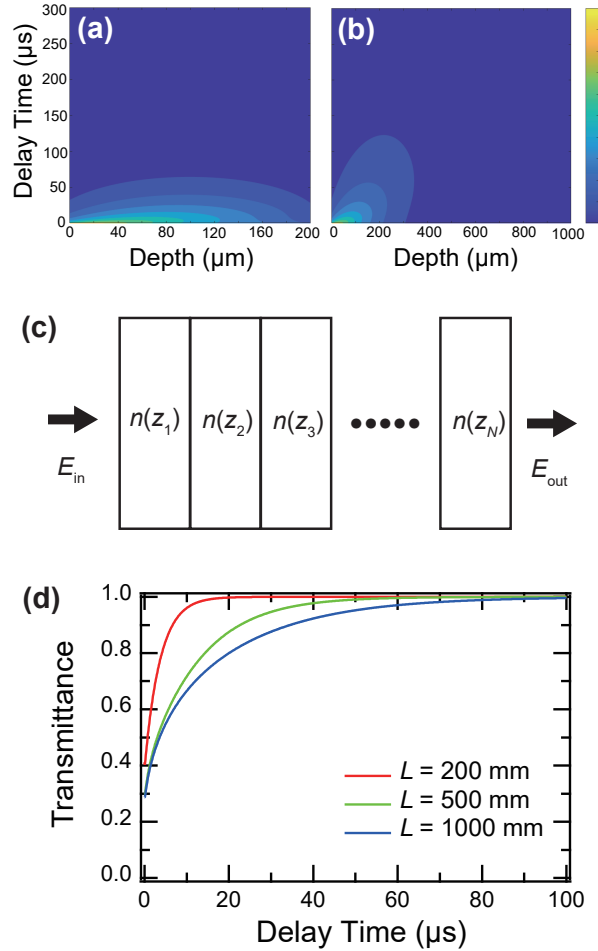

FIG. S1. Calculation results for the depth and temporal distributions of the carrier density for Si with  $L = 200$  (a) and  $1000 \mu\text{m}$  (b) based on the diffusion equations. (c) Schematic picture of the used model for simulating the transmittance of THz pulse. (d) Simulated results of the transmission of THz pulses for the sample thickness  $L = 200, 500$ , and  $1000 \mu\text{m}$

- 
- [1] C. A. Hoffman, K. Jarašiūnas, H. J. Gerritsen, and A. V. Nurmikko, Appl. Phys. Lett. **33**, 536 (1978).
  - [2] M. Rosling, H. Bleichner, P. Jonsson, and E. Nordlander, J. Appl. Phys. **76**, 2855 (1994).
  - [3] D. K. Schroder, IEEE Trans. Electron Devices **44**, 160 (1997).
  - [4] <https://www.cxro.lbl.gov/>
  - [5] A. G. Aberle, S. Glunz, and W. Warta, J. Appl. Phys. **71**, 4422 (1992).
  - [6] D. Grischkowsky, S. Keiding, M. van Exter, and Ch. Fattinger, J. Opt. Soc. Am. B **7**, 2006 (1990).
  - [7] T. Suzuki and R. Shimano, Phys. Rev. Lett. **109**, 046402 (2012).
